# Supplementary material for: Foundational Question Generation for Video Question Answering via an Embedding-Integrated Approach
Source: arXiv:2511.17618 source file (2025-11-18)
Supplement: Supplementary file 1 [file appendices.tex]

\input{chapters/apppendix_pseudocode}
